# Supplementary material for: Can Image Splicing and Copy-Move Forgery Be Detected by the Same Model? Forensim: An Attention-Based State-Space Approach
Source: arXiv:2602.10079 source file (2026-02-10)
Supplement: Supplementary file 1 [file X_suppl.tex]

% \clearpage
% \setcounter{page}{1}
% \maketitlesupplementary

\vspace{0.8em}
\begin{center}
{\large\bfseries Supplementary Material}
\end{center}
\vspace{0.5em}

In this supplementary document, we provide extended technical and experimental details supporting our main paper. \hyperref[sec:implementation]{Section~\ref*{sec:implementation}} outlines the Forensim model architecture and implementation details, including the backbone configuration, attention modules, fusion strategy, and training setup. \hyperref[sec:dataset_details]{Section~\ref*{sec:dataset_details}} presents a comprehensive overview of the datasets used for training and evaluation, including both synthetic and real-world forgery benchmarks. \hyperref[sec:loss]{Section~\ref*{sec:loss}} provides ablation studies on the loss functions, examining the individual and combined contributions of Cross-Entropy, Dice, Focal, and InfoNCE losses. \hyperref[sec:dataset_ablation]{Section~\ref*{sec:dataset_ablation}} explores the impact of dataset composition on generalization via ablation studies on the proposed \texttt{CMFD\_Anything} dataset. Finally, \hyperref[sec:comofod_attacks]{Section~\ref*{sec:comofod_attacks}} presents additional robustness analysis on CoMoFoD attacks, highlighting Forensim’s performance across diverse manipulation categories.

\noindent \textbf{Index Terms—} Copy-Move Forgery Detection (CMFD), Image Manipulation Detection and Localization (IMDL), State Space Models, Attention Mechanisms, Synthetic Datasets.

\section{Additional Implementation Details}
\label{sec:implementation}

\textbf{Backbone and Feature Extraction.}
Forensim uses the first four layers of a Vision Transformer (ViT) backbone pretrained with DINO on ImageNet. Input images are resized to $224 \times 224$ and passed through the backbone to extract hierarchical features \( V \in \mathbb{R}^{B \times N \times C} \), where \( B \) is batch size, \( N = H \times W \), and \( C = 384 \) is the embedding dimension.

\textbf{Similarity and Manipulation Attention.}
The extracted features are processed by two specialized attention modules: the Similarity State Space Attention (Sim\_Attn) and Multi-Level Manipulation State Space Attention (MSSA) modules, described in Sections 3.3 and 3.4 of the main text, respectively. The SSA module computes an affinity matrix using state-space recurrence with Rotary Positional Embeddings (RoPE), while the MSSA module integrates manipulation-aware information using multi-head self-attention with Locally Enhanced Positional Encoding (LePE)~\cite{dong2022cswin}.

\textbf{Fusion and Prediction.}
Features from SSA and MSSA are fused via a Non-Local Refinement (NLR) module, which performs global context aggregation based on similarity and manipulation maps. The fused representation is decoded using a lightweight convolutional head with SiLU activation to generate a pixel-level three-class segmentation mask (\textcolor{blue}{pristine}, \textcolor{green}{source}, \textcolor{red}{target}) and an image-level detection score.

\textbf{Loss Functions.}
We optimize Forensim using a weighted combination of pixel-wise Cross-Entropy Loss (CE), InfoNCE contrastive loss, Dice Loss (DL), and Focal Loss (FL). The overall loss is:
\[
\mathcal{L} = \lambda_{\text{CE}} \cdot \mathcal{L}_{\text{CE}} + \lambda_{\text{InfoNCE}} \cdot \mathcal{L}_{\text{InfoNCE}} + \lambda_{\text{DL}} \cdot \mathcal{L}_{\text{Dice}} + \lambda_{\text{FL}} \cdot \mathcal{L}_{\text{Focal}},
\]
with default weights: $\lambda_{\text{CE}}=1.0$, $\lambda_{\text{InfoNCE}}=0.1$, $\lambda_{\text{DL}}=1.0$, and $\lambda_{\text{FL}}=0.5$. Ablations for loss terms are discussed in Section~\ref{tab:loss_ablation}.

\textbf{Contrastive Supervision.}
Positive pairs are sampled from source-target regions, and negatives from pristine patches. In each batch, we randomly sample 64 positive and 256 negative pairs. Contrastive training encourages discriminative feature learning for manipulated vs. pristine regions.

\textbf{Training Configuration.}
Training is performed in PyTorch on an NVIDIA RTX A5000 GPU with 24GB memory. We use the AdamW optimizer with a cyclic learning rate scheduler ranging from $10^{-3}$ to $10^{-5}$ and StepLR decay by 0.5 every 10 epochs. Models are trained for 100 epochs with a batch size of 64, sampling 100K images per epoch. Early stopping is applied based on validation loss.

\textbf{Evaluation Protocol.}
Models are evaluated using both pixel-level and image-level metrics. Pixel-level performance includes precision, recall, F1, MCC, AUC, and Balanced Accuracy (BAcc), computed using three-class RGB masks. Following prior works~\cite{wu2019mantra, islam2020doa}, we apply a 200-pixel threshold to suppress small false positives. Image-level scores are derived by averaging segmentation confidence. Additionally, we reported the metric performance for Pristine (P), Source (S) and Target (T) regions for CMFD pixel-level evaluations in Table 2 of the main text.

\section{Details on Datasets}
\label{sec:dataset_details}

\begin{table*}[t]
    \centering
    \footnotesize
    \caption{
    Summary of image manipulation datasets used for training and evaluation. Datasets are grouped by use case: training on synthetic manipulations, and testing on natural image forensics (IMDL). Manipulation types: splicing and copy-move for natural image forensics.
    }
    \label{tab:manip_datasets}
    \begin{tabular}{l|c|c|c|c}
        \toprule
        \textbf{Dataset Name} & \textbf{Real} & \textbf{Fake} & \textbf{Splicing} & \textbf{Copy-move} \\
        \midrule
        \multicolumn{5}{c}{\textbf{Training, Validation, Test (8:1:1) : Synthetic Manipulations (CMFD on Natural Images)}} \\
        \midrule
        Casia CMFD~\cite{dong2013casia} & 1313     & 1313    & \ding{55} & \ding{51} \\
        CoMoFoD CMFD~\cite{tralic2013comofod} & 0     & 5000    & \ding{55} & \ding{51} \\
        Synthetic Images from MSCOCO~\cite{lin2014microsoft} and SUN2012~\cite{xiao2010sun} for USC-ISI CMFD~\cite{wu2018busternet}       & 0     & 100K    & \ding{55} & \ding{51} \\
        Synthetic Images from Segment Anything~\cite{kirillov2023segment} for CMFD\_Anything (Ours) & 100K     & 200K    & \ding{51} & \ding{51} \\
        \midrule
        \multicolumn{5}{c}{\textbf{Test: Natural Image Forensics (IMDL)}} \\
        \midrule
        CASIA~\cite{dong2013casia}                                  & 7,491  & 5,105   & \ding{51} & \ding{51} \\
        Coverage~\cite{wen2016coverage}                             & 100    & 100     & \ding{51} & \ding{55} \\
        Columbia~\cite{ng2009columbia}                              & 183    & 180     & \ding{51} & \ding{55} \\
        NIST16~\cite{NimbleCh33:online}                              & 160    & 160     & \ding{51} & \ding{51} \\
        \bottomrule
    \end{tabular}
\end{table*}

\hyperref[tab:manip_datasets]{Table~\ref*{tab:manip_datasets}} summarizes the datasets used for training and evaluation. For synthetic CMFD training, we include datasets with copy-move manipulations such as CASIA CMFD, CoMoFoD CMFD, USC-ISI CMFD, and our \texttt{CMFD\_Anything}, which uniquely includes both copy-move and splicing manipulations synthesized using masks from the Segment Anything model~\cite{kirillov2023segment}. It is to be noted that our \texttt{CMFD\_Anything} is the only dataset including pristine images for CMFD training. 

We evaluated the Forensim model on three benchmark CMFD datasets—USC-ISI CMFD~\cite{wu2018busternet}, CoMoFoD~\cite{tralic2013comofod}, and CASIA CMFD~\cite{dong2013casia}—as well as the test split of our proposed \texttt{CMFD\_Anything} dataset and four baseline IMDL evaluation datasets: NIST16~\cite{NimbleCh33:online}, Columbia~\cite{ng2009columbia}, Coverage~\cite{wen2016coverage}, and CASIA~\cite{dong2013casia}. The USC-ISI CMFD dataset consists of 80K training images and 10K each for validation and testing. CoMoFoD contains 5,000 forged images generated from 200 base images across 25 manipulation categories, combining five manipulation types and five post-processing operations. CASIA CMFD includes 1,313 forged and 1,313 authentic images, totaling 2,626 samples.

For IMDL evaluation, we focus on datasets that contain real-world manipulations: CASIA, Columbia, Coverage, and NIST16. These datasets span both splicing and copy-move tasks, offering a robust benchmark for assessing generalization to natural image forensics. Notably, while some datasets like Columbia and Coverage contain only splicing, others such as NIST16 and CASIA include both manipulation types, supporting a comprehensive evaluation across forgery categories.

\begin{table*}[t]
    \centering
    \caption{Ablation study on loss functions. Pixel-level metrics on the CMFD\_Anything test set that include MCC (Matthews Correlation Coefficient), F1 score (Target class), AUC (Area Under the Curve), and BAcc (Balanced Accuracy). CE = Cross-Entropy, INCE = InfoNCE, DL = Dice Loss, FL = Focal Loss.}
    \vspace{-2mm}
    \setlength{\tabcolsep}{4pt}
    \begin{tabular}{l|c|c|c|c}
        \toprule
        \textbf{Loss Function} & \textbf{MCC~\cite{chicco2020advantages}} & \textbf{F1 (Target)} & \textbf{AUC} & \textbf{BAcc} \\
        \midrule
        CE + DL      & 0.652 & 0.600 & 0.689 & 0.796 \\
        CE + FL      & 0.638 & 0.590 & 0.684 & 0.782 \\
        CE only      & 0.611 & 0.572 & 0.678 & 0.776 \\
        INCE only    & 0.589 & 0.548 & 0.665 & 0.761 \\
        CE + INCE    & \textbf{0.681} & \textbf{0.624} & \textbf{0.700} & \textbf{0.812} \\
        \bottomrule
    \end{tabular}
    \vspace{-2mm}
    \label{tab:loss_ablation}
\end{table*}

\begin{table*}[t]
    \centering
    \caption{Dataset ablation study. All models are evaluated on the CMFD\_Anything test set with Forensim. We vary the training composition by dataset and manipulation type. Performance improves with diverse forgery exposure.}
    \vspace{-2mm}
    \setlength{\tabcolsep}{5pt}
    \begin{tabular}{l|c|c|c|c}
        \toprule
        \textbf{Training Data} & \textbf{MCC} & \textbf{F1 (Target)} & \textbf{AUC} & \textbf{BAcc} \\
        \midrule
        CASIA~\cite{dong2013casia} only (Splicing)         & 0.418 & 0.316 & 0.598 & 0.683 \\
        CASIA~\cite{dong2013casia} only (Copy-Move)        & 0.401 & 0.302 & 0.587 & 0.671 \\
        CASIA~\cite{dong2013casia} only (Removal)          & 0.406 & 0.308 & 0.592 & 0.677 \\
        CoMoFoD~\cite{tralic2013comofod} only (Copy-Move)  & 0.389 & 0.292 & 0.579 & 0.664 \\
        CASIA~\cite{dong2013casia} + CoMoFoD~\cite{tralic2013comofod} & 0.510 & 0.374 & 0.623 & 0.712 \\
        CMFD\_Anything only (Copy-Move)                    & 0.622 & 0.590 & 0.682 & 0.766 \\
        All Combined for Forensim training                                & \textbf{0.681} & \textbf{0.624} & \textbf{0.700} & \textbf{0.812} \\
        \bottomrule
    \end{tabular}
    \vspace{-2mm}
    \label{tab:dataset_ablation}
\end{table*}

\section{Additional Ablation Study on Forensim Loss Functions}
\label{sec:loss}

\section*{Cross-Entropy Loss for Three Classes}

The Cross-Entropy Loss~\cite{fisher1936use} for a multi-class classification problem with three classes (pristine, source, target) is given by:

\vspace{-10px}
\begin{equation}
\mathcal{L}_{\text{CE}} = - \frac{1}{N} \sum_{i=1}^{N} \sum_{c=1}^{C} y_{i,c} \log(p_{i,c})
\end{equation}
\vspace{-10px}

\noindent where:
\begin{itemize}
    \item \( N \) is the number of samples (images).
    \item \( C \) is the number of classes (in this case, 3 classes: pristine, source, and target).
    \item \( y_{i,c} \) is the ground-truth label for sample \( i \) and class \( c \) (binary: 1 if the sample belongs to the class, otherwise 0).
    \item \( p_{i,c} \) is the predicted probability for sample \( i \) and class \( c \) (obtained from the model’s output).
\end{itemize}

This formula computes the loss by summing over all samples and classes, applying the logarithm to the predicted probabilities, and averaging over the batch size \( N \).

\section*{InfoNCE Loss for Three Classes}
The InfoNCE loss~\cite{oord2018representation} for a contrastive learning setting with three classes (pristine, source, target) is given by:

\vspace{-10px}
\begin{equation}
\begin{aligned}
\mathcal{L}_{\text{InfoNCE}} = \\
- \frac{1}{N} \sum_{i=1}^{N} \log 
\frac{ \exp(\mathbf{z}_i \cdot \mathbf{z}_i^+ / \tau)}{
\exp(\mathbf{z}_i \cdot \mathbf{z}_i^+ / \tau) + 
\sum_{j=1}^{M} \exp(\mathbf{z}_i \cdot \mathbf{z}_j^- / \tau)}
\end{aligned}
\end{equation}
\vspace{-10px}

\noindent where:
\begin{itemize}
    \item \( N \) is the number of samples (images).
    \item \( \mathbf{z}_i \) is the feature vector for sample \( i \).
    \item \( \mathbf{z}_i^+ \) is the feature vector of the positive sample (e.g., source-target pair for \( i \)).
    \item \( \mathbf{z}_j^- \) is the feature vector of the negative samples (e.g., other regions or non-related images).
    \item \( \tau \) is the temperature parameter that controls the smoothness of the softmax.
    \item \( M \) is the number of negative samples (2 in this case, for each positive pair).
\end{itemize}

This loss function minimizes the distance between the positive pairs while maximizing the distance from the negative pairs, thereby improving the model’s ability to distinguish between the different image regions.

\section*{Dice Loss}
The Dice Loss~\cite{milletari2016v}, often used for evaluating segmentation tasks, is given by:

\vspace{-10px}
\begin{equation}
\mathcal{L}_{\text{Dice}} = 1 - \frac{2 \sum_{i=1}^{N} p_i g_i}{\sum_{i=1}^{N} p_i + \sum_{i=1}^{N} g_i}
\end{equation}
\vspace{-10px}

\noindent where:
\begin{itemize}
    \item \( p_i \) is the predicted probability (or binary prediction) for pixel \( i \).
    \item \( g_i \) is the ground truth (binary) value for pixel \( i \).
    \item \( N \) is the total number of pixels in the image.
\end{itemize}

The Dice Loss is based on the Dice coefficient, a measure of overlap between two binary sets, and is especially useful when dealing with imbalanced classes. It penalizes differences between the predicted and ground truth segmentation masks by maximizing the overlap between them.

\begin{table*}[t]
    \centering
    \setlength{\tabcolsep}{3.5pt}
    \scalebox{0.92}{
    \begin{tabular}{l|cccc|cccc|cccc|cccc|cccc}
        \toprule
        \multirow{2}{*}{\textbf{Method}}
        & \multicolumn{4}{c|}{\textbf{CASIA v1}} 
        & \multicolumn{4}{c|}{\textbf{Columbia}} 
        & \multicolumn{4}{c|}{\textbf{DSO-1}} 
        & \multicolumn{4}{c|}{\textbf{NIST16}} 
        & \multicolumn{4}{c}{\textbf{AVG}} \\
        \cmidrule(lr){2-5}\cmidrule(lr){6-9}\cmidrule(lr){10-13}\cmidrule(lr){14-17}\cmidrule(lr){18-21}
        & Fb & Wa & Wb & Wc & Fb & Wa & Wb & Wc & Fb & Wa & Wb & Wc & Fb & Wa & Wb & Wc & Fb & Wa & Wb & Wc \\
        \midrule
        IF-OSN~\cite{wu2022robust}          
            & .513 & .524 & .507 & .454 
            & .741 & .752 & .756 & .760 
            & .484 & .395 & .416 & .414 
            & .315 & .302 & .292 & .282 
            & .513 & .493 & .493 & .478 \\
        CAT-Net v2~\cite{kwon2021cat}      
            & .681 & .508 & .469 & .206 
            & \textbf{.964} & \textbf{.952} & \textbf{.958} & \textbf{.903} 
            & .310 & .247 & .240 & .237 
            & .219 & .238 & .243 & .244 
            & .544 & .486 & .478 & .398 \\
        MVSS-Net~\cite{chen2021image}         
            & .469 & .444 & .480 & .339 
            & .752 & .747 & .758 & .752 
            & .356 & .308 & .354 & .329 
            & .305 & .252 & .300 & .269 
            & .471 & .438 & .473 & .422 \\
        TruFor~\cite{guillaro2023trufor}                
            & \underline{.716} & \underline{.713} & \underline{.676} & \underline{.615} 
            & .797 & .798 & .835 & .820 
            & \textbf{.685} & \textbf{.465} & \textbf{.515} & \textbf{.469} 
            & \underline{.338} & \underline{.384} & \underline{.308} & \underline{.358} 
            & \underline{.634} & \underline{.590} & \underline{.584} & \underline{.566} \\
        \textbf{Forensim}            
            & \textbf{.729} & \textbf{.722} & \textbf{.685} & \textbf{.628} 
            & \underline{.806} & \underline{.806} & \underline{.842} & \underline{.828} 
            & \underline{.670} & \underline{.452} & \underline{.502} & \underline{.455} 
            & \textbf{.346} & \textbf{.392} & \textbf{.315} & \textbf{.366} 
            & \textbf{.638} & \textbf{.593} & \textbf{.586} & \textbf{.569} \\
        \bottomrule
    \end{tabular}}
    \caption{Pixel-level F1 (fixed threshold of 0.5) on images uploaded to social networks: Facebook (Fb), WhatsApp (Wa), Weibo (Wb), and WeChat (Wc). \textbf{Bold} = Best, \underline{Underline} = Second-Best.}
    \label{tab:social_f1}
\end{table*}

\begin{figure*}
    \centering
    \includegraphics[width=\textwidth]{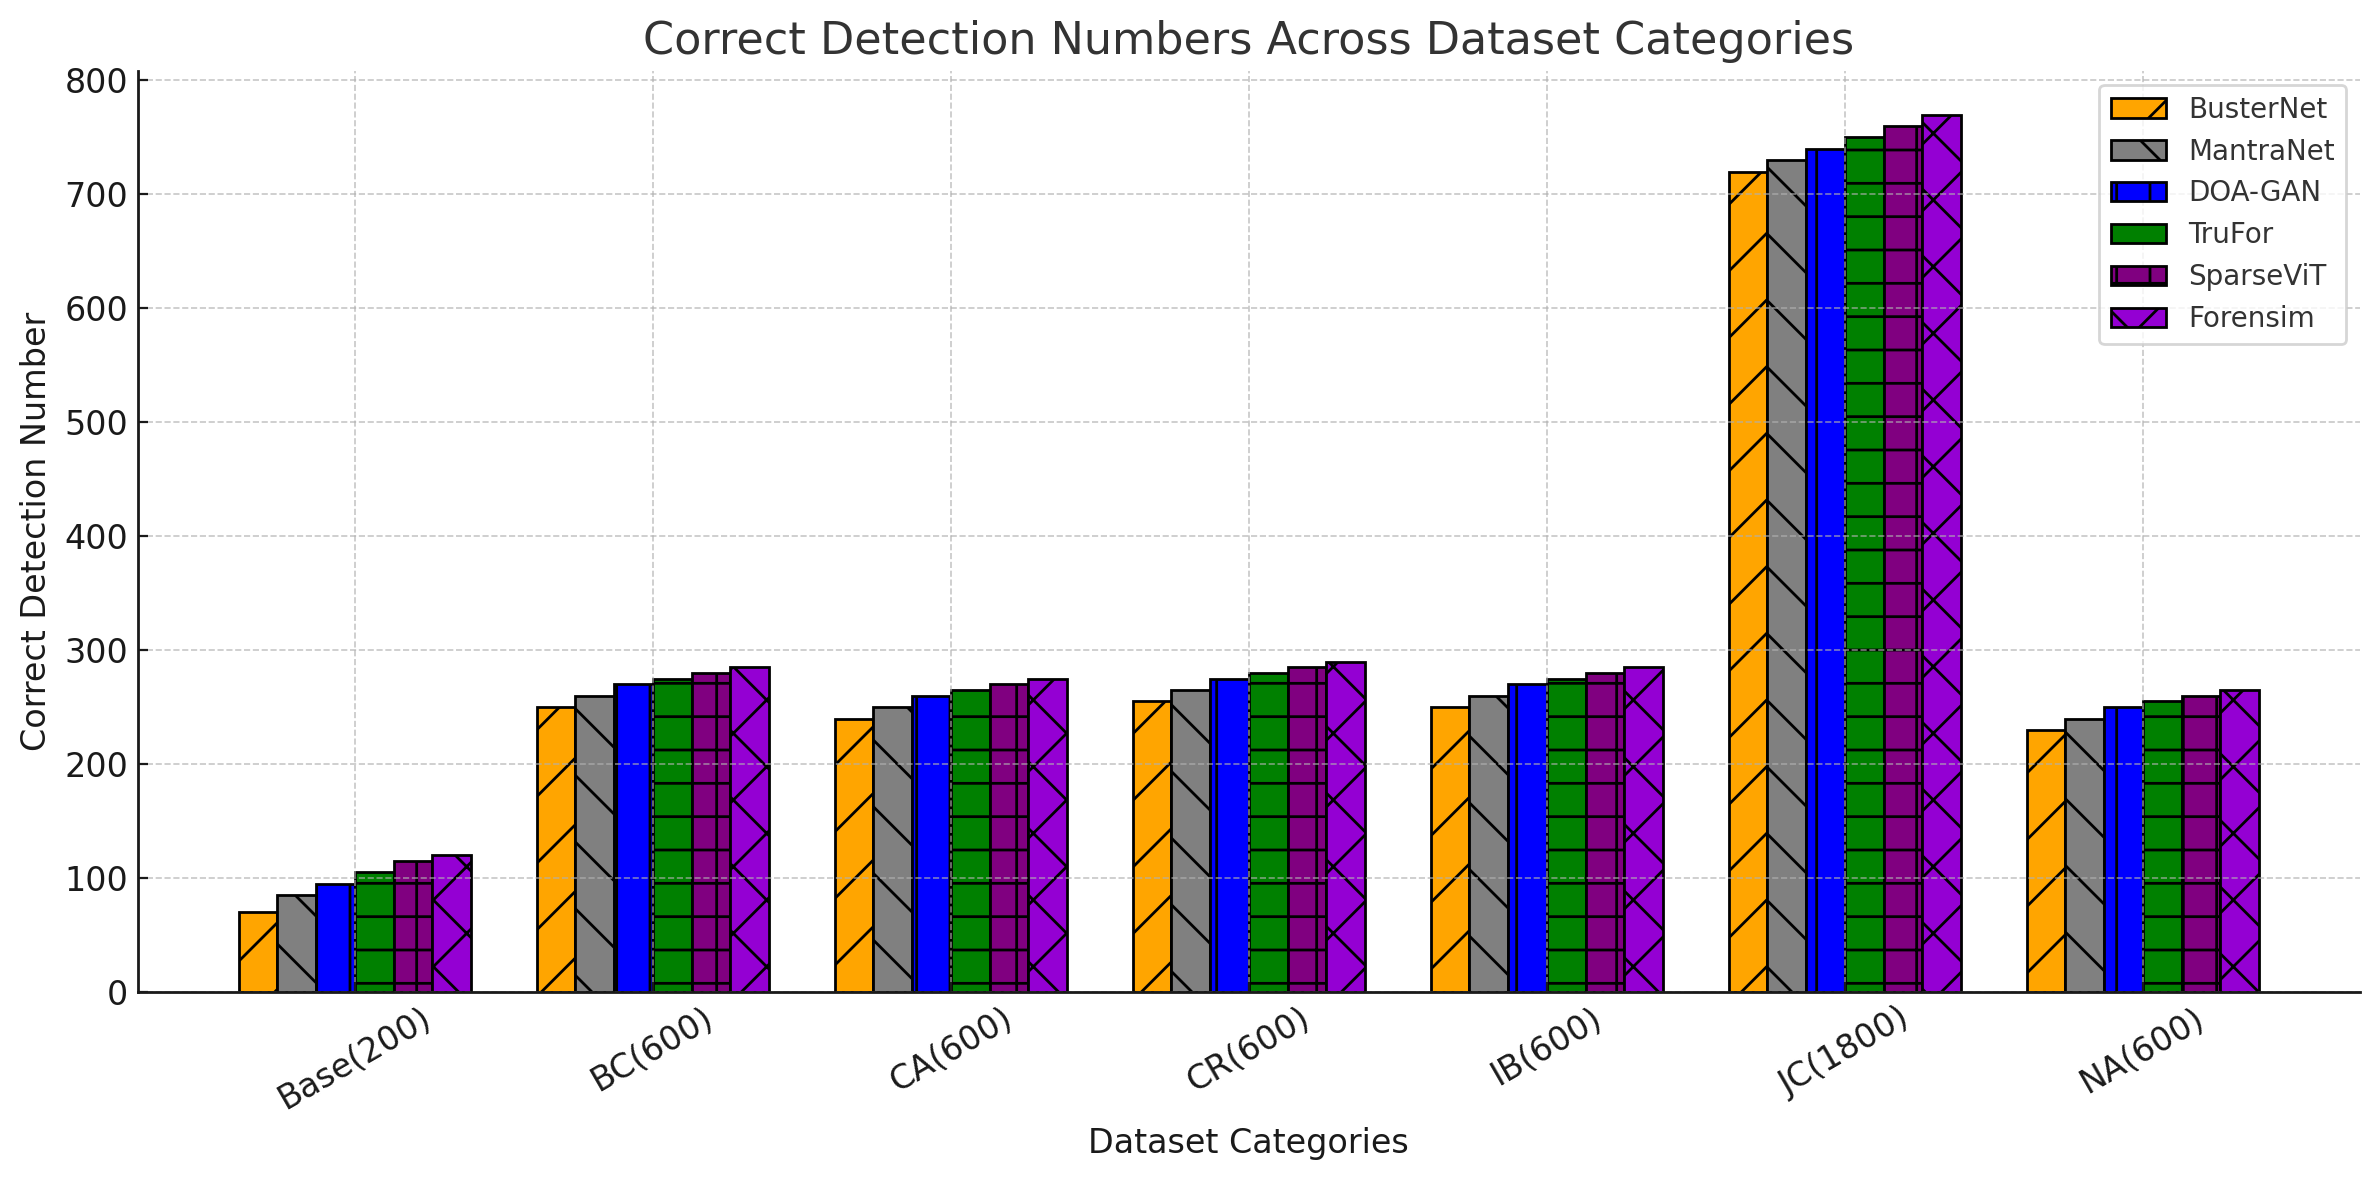}
    \caption{Comparison of correct detection numbers across different dataset categories for various forgery detection methods. The models compared include Adaptive-Seg, DenseField, BusterNet, DOA-GAN, and Forensim. DOA-GAN outperforms previous methods in most categories, while Forensim achieves the highest detection rate, slightly surpassing DOA-GAN. Each method is represented with a unique color and texture for clarity.}
    \label{fig:comofod_attacks}
\end{figure*}

\section*{Focal Loss}
Focal Loss~\cite{lin2017focal}, a modification of cross-entropy loss, is defined as:

\vspace{-10px}
\begin{equation}
\mathcal{L}_{\text{Focal}} = - \alpha (1 - p_t)^\gamma \log(p_t)
\end{equation}
\vspace{-10px}

\noindent where:
\begin{itemize}
    \item \( p_t \) is the predicted probability for the true class, i.e., \( p_t = p \) for the positive class and \( p_t = 1 - p \) for the negative class.
    \item \( \alpha \) is a weighting factor to adjust for class imbalance, typically set to 0.25.
    \item \( \gamma \) is the focusing parameter, commonly set to 2, which controls the down-weighting of well-classified examples.
    \item \( p \) is the predicted probability of the positive class.
\end{itemize}

The Focal Loss introduces a modulating factor \( (1 - p_t)^\gamma \) that reduces the relative loss for well-classified examples, thereby focusing training on hard, misclassified examples. It is particularly useful in tasks with class imbalance.

\noindent\textbf{Discussion. }Forensim leverages a combination of complementary loss functions to enhance accuracy and robustness in copy-move forgery detection (CMFD). Cross-Entropy Loss is employed for multi-class pixel classification, enabling the model to distinguish pristine, source, and target regions. InfoNCE Loss maximizes mutual information between similar patches by pulling positive pairs closer and pushing apart negative pairs, aiding in manipulation-aware representation learning. Dice Loss further improves segmentation quality by optimizing the overlap between predicted and ground-truth masks, while Focal Loss addresses class imbalance by emphasizing harder-to-classify pixels. The effectiveness of each component is demonstrated in the ablation study (\hyperref[tab:loss_ablation]{Tab.~\ref*{tab:loss_ablation}}), where the combination of Cross-Entropy and InfoNCE achieves the best trade-off across all metrics. Among them, Balanced Accuracy (BAcc) is particularly relevant in imbalanced settings, and is computed as the mean class-wise recall: $\text{BAcc} = \frac{1}{C} \sum_{c=1}^{C} \frac{\text{TP}_c}{\text{TP}_c + \text{FN}_c}$, where $C$ is the number of classes and TP/FN denote true positives and false negatives for class $c$. Together, these loss functions enable Forensim to localize source and target regions more precisely, even in challenging complex forgery scenarios.

\section{Additional Ablation Study on CMFD\_Anything Dataset}
\label{sec:dataset_ablation}

To assess the impact of dataset composition on model performance, we conduct a dataset ablation study across different manipulation types and sources. As shown in \hyperref[tab:dataset_ablation]{Tab.~\ref*{tab:dataset_ablation}}, models trained exclusively on CASIA~\cite{dong2013casia} or CoMoFoD~\cite{tralic2013comofod} achieve limited performance, with maximum F1 scores of 31.6\% and 29.2\%, respectively. This highlights their limited diversity and domain coverage. Incorporating CMFD\_Anything as a training source boosts generalization, while combining CASIA and CoMoFoD yields moderate improvements. The best performance is achieved when all datasets are combined, confirming that diverse training data significantly enhances the model's robustness across different manipulation types.

\vspace{-6px}
\section{Additional Robustness Analysis on CoMoFoD Attacks}
\label{sec:comofod_attacks}

\hyperref[fig:comofod_attacks]{Figure~\ref*{fig:comofod_attacks}} shows the number of correctly detected images across seven attack categories in the CoMoFoD dataset, where a prediction is considered correct if its pixel-level F1 score exceeds 30\%. We compare several state-of-the-art copy-move forgery detection models, including BusterNet~\cite{wu2018busternet}, MantraNet~\cite{wu2019mantra}, DOA-GAN~\cite{islam2020doa}, TruFor~\cite{guillaro2023trufor}, SparseViT~\cite{su2025can}, and our proposed Forensim. Forensim consistently outperforms all baselines across most attack categories—including challenging ones like Joint Compression (JC) and Noised Affine (NA)—demonstrating its strong robustness to various post-processing operations. Notably, SparseViT and TruFor also show strong performance, but Forensim achieves the highest number of correctly detected images overall, highlighting its effectiveness in real-world manipulation scenarios.

\vspace{-6px}
\section{Additional Robustness Analysis on Social-Network Uploads.}
As illustrated in Table~\ref{tab:social_f1}, \textit{Forensim} performs consistently better than other baselines across platforms (Fb/Wa/Wb/Wc) and datasets, indicating robustness to social-media degradations (pixel-level F1 at a fixed 0.5 threshold).
